# Supplementary material for: Attributing AUC-ROC to Analyze Binary Classifier Performance
Source: arXiv:2205.11781 source file (2022-05-24)
Supplement: Supplementary file 1 [file appendix.tex]

\begin{table*}[]
\begin{tabular}{|l|l|l|l|l|l|l|}
\hline
Slice               & CE Loss RF & CE Loss LR & GINI RF      & GINI LR  & AUC RF & AUC LR      \\ \hline
All data            & 0.48       &   0.50     & 0.31         & 0.32     &   0.70  & 0.64             \\ \hline
Debt Consolidation  & 0.49       &   0.51     & 0.32         & 0.34     &   0.70  & 0.64           \\ \hline
Vacation            & 0.50       &   0.53     & 0.32         & 0.31     &   0.68  & 0.62            \\ \hline
Major Purchase      & 0.47       &   0.50     & 0.31         & 0.30     &   0.72  & 0.67        \\ \hline
\end{tabular}
\caption{A logistic regression model (LR) and a random forest model (RF) trained on the same data and features are evaluated on different \textit{Loan Purpose} segments. The random forest outperforms the logistic regression model on all slices and metrics. The patterns discussed in Section~\ref{sec:misleading} are not present. \label{tab:loss-example-lending}}
\end{table*}

\begin{figure}[h]
\caption{AUC Attributions are well-correlated with CE Loss for each class separately in the Census dataset. But items from the negative class participate in more pairs than items from the positive class, and as a result receive a higher AUC Attribution.}
\centering
\includegraphics[width=0.5\textwidth]{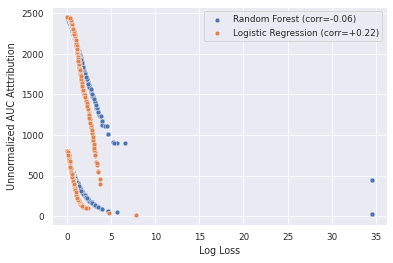}
\end{figure}

\begin{figure}[h]
\caption{Normalized AUC Attributions are well-correlated with CE Loss in the Census dataset. The normalization matches the scales of AUC Attributions for positive and negative items.}
\centering
\includegraphics[width=0.5\textwidth]{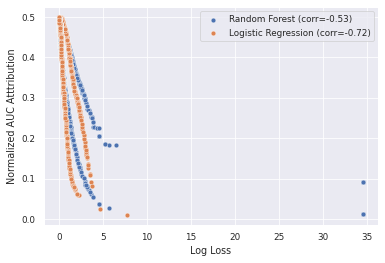}
\end{figure}

\begin{figure}[h]
\caption{AUC Attributions are well-correlated with GINI Impurity for each class separately in the Lending dataset. But items from the negative class participate in more pairs than items from the positive class, and as a result receive a higher AUC Attribution.}
\centering
\includegraphics[width=0.5\textwidth]{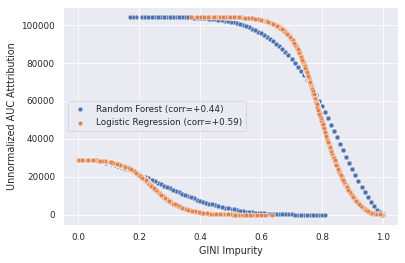}
\end{figure}

\begin{figure}[h]
\caption{Normalized AUC Attributions are well-correlated with GINI Impurity in the Lending dataset. The normalization matches the scales of AUC Attributions for positive and negative items.}
\centering
\includegraphics[width=0.5\textwidth]{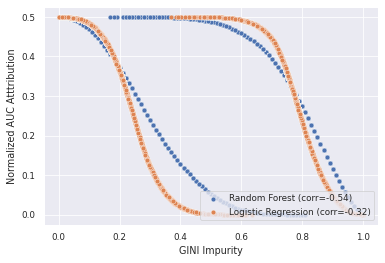}
\end{figure}

\begin{figure}[h]
\caption{AUC Attributions are well-correlated with CE Loss for each class separately in the Lending dataset. But items from the negative class participate in more pairs than items from the positive class, and as a result receive a higher AUC Attribution.}
\centering
\includegraphics[width=0.5\textwidth]{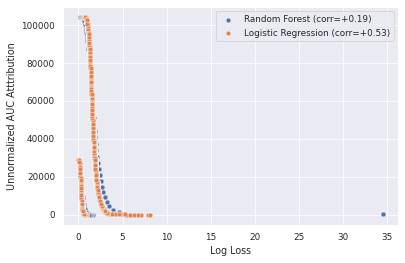}
\end{figure}
\begin{figure}[h]
\caption{Normalized AUC Attributions are well-correlated with CE Loss in the Lending dataset. The normalization matches the scales of AUC Attributions for positive and negative items.}
\centering
\includegraphics[width=0.5\textwidth]{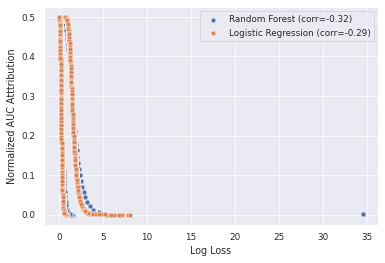}
\end{figure}

\begin{figure*}[h]
\caption{}
\centering
\includegraphics[width=\textwidth]{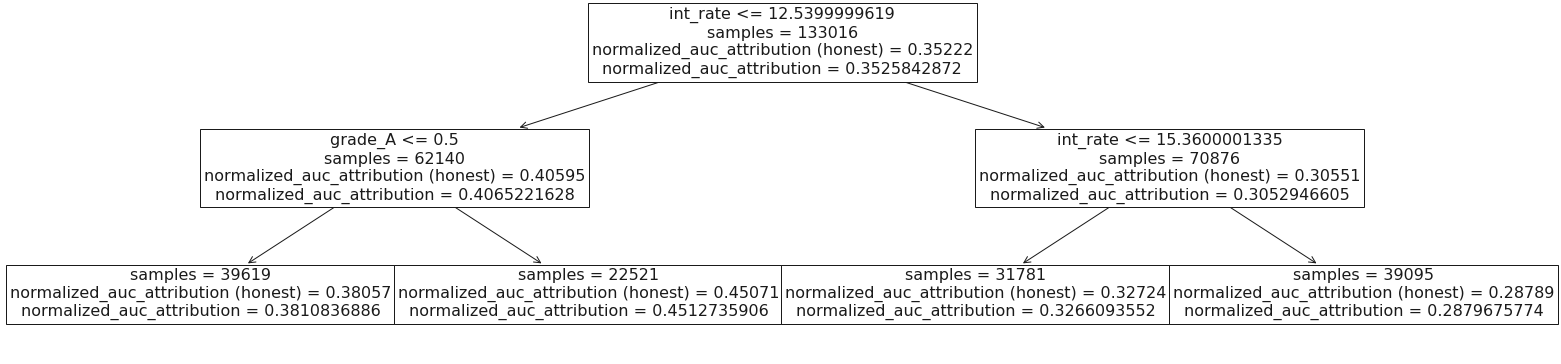}
\label{fig:forest-tree}
\end{figure*}

\begin{table*}[]
\begin{tabular}{|l|l|l|l|}
\hline
Slice                     & Mean CE Loss    & Mean GINI Impurity    & Mean AUC Attribution  \\ \hline
All data                  &     0.50        &    0.32               &     0.32              \\ \hline
interest rate <= 12.54        &     0.38        &    0.25               &     0.36      \\ \hline
interest rate > 12.54    &     0.61        &    0.39               &     0.29      \\ \hline   
\end{tabular}
\begin{tabular}{|l|l|l|l|}
\hline
Slice                     & Mean CE Loss    & Mean GINI Impurity    & Mean AUC Attribution  \\ \hline
All data                  &     0.48        &    0.31               &     0.35  \\ \hline
interest rate <= 12.54         &     0.36        &    0.21               &     0.41     \\ \hline
interest rate > 12.54          &     0.58        &    0.40               &     0.21      \\ \hline   
\end{tabular}
\caption{Segments with divergent model performance (top: logistic regression, bottom: random forest) are identified. All three metrics identify similar patterns: both models perform relatively poorly on the $interest\_rate > 12.54$ segment.}
\end{table*}

\begin{figure*}[h]
\caption{}
\centering
\includegraphics[width=\textwidth]{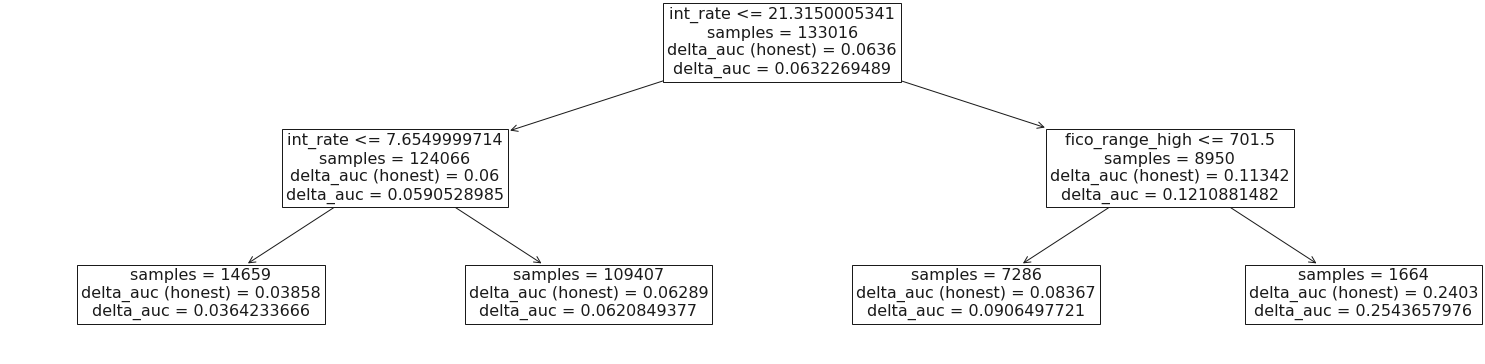}
\label{fig:delta-tree}
\end{figure*}

\begin{figure}[h]
\caption{AUC computed for the logistic regression model on \textit{Relationship} slices in the Census dataset. Diagonal entries correspond to the fraction of correctly ordered pairs where both items belong to the same category. The off-diagonal entries similarly correspond to pairs where the items belong to different categories. We point out the variety in the model's performance across these slices.\label{fig:cross-auc-census}}
\centering
\includegraphics[width=0.5\textwidth]{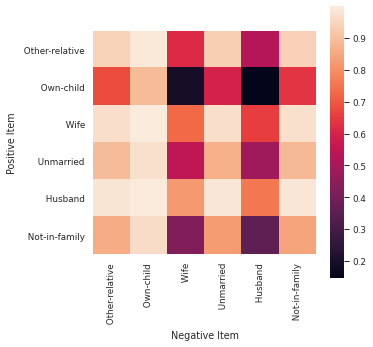}
\end{figure}
